# Supplementary material for: Deep Generative Modeling for Scene Synthesis via Hybrid Representations
Source: arXiv:1808.02084 source file (2018-08-06)
Supplement: Supplementary file 1 [file 09_appendix.tex]

\section{Stein Discrepancy}
\label{Sec:Distance}

In this section, we provide a detailed introduction of the proposed Stein discrepancy measurement used in this paper.
We start with the Stein operator, which provides the foundation for our continuous formulation.
\begin{defn}
Given a function $f(\bs{x})$ and a smooth probability distribution $p(\bs{x})$ over a space $\Omega$, we define the Stein operator on $f(\bs{x})$ as
$$
\set{A}_{p}f(\bs{x}):= \nabla \log(p(\bs{x}))f(\bs{x}) + \nabla_{\bs{x}} f(\bs{x}).
$$
\end{defn}

We then define the notion of the \textsl{Stein} class of a probability distribution, which will be used later:
\begin{defn}
Given a space $\Omega$ and probability distribution $p(\bs{x})$ over $\Omega$, we say a function $f(\bs{x})$ is in the Stein class of $p(\bs{x})$ if
$$
\int_{\Omega}\nabla_{\bs{x}}(f(\bs{x})p(\bs{x})) = 0.
$$
\label{Defn:Stein:Class}
\end{defn}
In the case $\Omega = \R^d$, one condition that holds for Definition (\ref{Defn:Stein:Class}) is that $f(\bs{x})p(\bs{x}) = 0$ when $\|\bs{x}\|\rightarrow \infty$. For example, the kernel function $k(\bs{x},\bs{z}) = \exp(-\frac{\|\bs{x}-\bs{z}\|^2}{h})$ for fixed $\bs{z}$ is the Stein class of the normal distribution.

Now we introduce an important property of the Stein operator:
\begin{prop}
If $f(\bs{x})$ is in the Stein class of $p(\bs{x})$, then
\begin{equation}
E_{x\sim p}\big(\set{A}_{p}f\big)(\bs{x}) := \int_{\Omega}\set{A}_{p}f(\bs{x}) \cdot p(\bs{x}) d\bs{x} = 0.
\label{Eq:Stein}
\end{equation}
\end{prop}
\noindent\textsl{Proof:}
\begin{align}
E_{x\sim p}\big(\set{A}_{p}f\big)(\bs{x}) & = \int_{\Omega}\big(\nabla \log{p(\bs{x})} f(\bs{x}) + \nabla f(\bs{x})\big)p(\bs{x}) d\bs{x}  \nonumber \\
& = \int_{\Omega}\big(\nabla p(\bs{x}) f(\bs{x}) + \nabla f(\bs{x}) p(\bs{x}) \big)d\bs{x} \nonumber \\
& = \int_{\Omega} \nabla_{\bs{x}}(p(\bs{x})f(\bs{x}))d\bs{x} = 0.
\end{align}
\qed

(\ref{Eq:Stein}) provides a powerful tool to access the difference between two distributions $p$ and $q$, namely, $E_{x\sim q}\big(\set{A}_{p}f\big)(\bs{x}) =0$ would not hold when $q \neq p$. To convert this intuition into a distance measure, we utilize a positive definite kernel function $k(\bs{x}, \bs{x}')$ and define:
\begin{equation}
\set{D}(q||p) := E_{\overline{\bs{x}}\sim p}\|E_{x\sim q}A_{p}k(\bs{x},\overline{\bs{x}})\|^2.
\label{Eq:D}
\end{equation}

We can show that under mild conditions of $p$ and $q$. $\set{D}(q||p) = 0$ if and only if $p = q$, which means $\set{D}$ provides a meaningful distance measure between probability distributions. To formalize this, we need to define the reproducing kernel Hilbert space of a kernel:
\begin{definition}
Let $k(\bs{x},\bs{x}'):\Omega \times \Omega \rightarrow \R^{+}$ be a positive definite kernel. The reproducing kernel Hilbert space (RKHS) $\set{H}$ of $k(\bs{x},\bs{x}')$ is the closure of the linear span $\{f:f(\bs{x}):= \sum_{i=1}^{m}a_i k(\bs{x}, \bs{x}_i), a_i \in \R, m \geq 0, \bs{x}\in \Omega\}$, equipped with inner products $<f.g>_{H} = \sum_{ij}a_i b_j k(\bs{x}_i, \bs{x}_j)$ for $g(\bs{x}) = \sum_i b_i k(\bs{x}, \bs{x}_i)$.
\end{definition}

\begin{prop}
Given a positive definite kernel $k$ and the associated reproducing kernel Hilbert space $\set{H}$. Suppose $p,q \in \set{H}$. Then
$$
\set{D}(q||p) = 0 \qquad \textup{iff} \qquad q = p.
$$
\label{Prop:1}
\end{prop}

\noindent\textsl{Proof:} Since $k(x,x')$ is in the stain class of $p$, $k(\cdot,\bar{x})$ is in the stain class of $p$ which implies $E_{x\sim p}\set{A}_pk(x,\bar{x})=0$ for all $\bar{x}\in \Omega$. Therefore, if $p=q$, $\set{D}(q\|p)=0$. We only need to show $p=q$ if $\set{D}(q\|p)=0$.

Note that $k(x,x')$ is in the Stein class of $q$ and $q$ is a smooth density function. We have for any fixed $\bar{x}\in\Omega$,
\begin{align}
   &\int_{\Omega}\nabla_x(k(x,\bar{x})q(x))dx\nonumber\\
   =&\int_{\Omega}(k(x,\bar{x})\nabla_x \log q(x)+\nabla_x k(x,\bar{x}))q(x) dx=0
   \label{Eq:A1}
\end{align}
By applying Proposition(1) and (\ref{Eq:A1}), we have
\begin{align}
   &E_{x\sim q}\set{A}_pk(x,\bar{x})\nonumber\\
   =&\int_{\Omega}\set{A}_pk(x,\bar{x})q(x)dx\nonumber\\
   =&\int_{\Omega}((\nabla_x\log p(x))k(x,\bar{x})+\nabla_xk(x,\bar{x}))q(x) dx\nonumber\\
   =&\int_{\Omega}(\nabla_x\log p(x)-\nabla_x\log q(x))k(x,\bar{x})q(x) dx.\nonumber
\end{align}

We can do spectral decomposition of $k(x,x')$, as implied by Mercer's theorem, to get
$$k(x,x')=\sum_j\lambda_je_j(x)e_j(x'),$$
where $\{e_j\}\{\lambda_j\}$ are the orthonormal eigenfunctions and positive eigenvalues of $k(x,x')$, satisfying $\int_\Omega e_i(x)e_j(x)dx=\mathbb{I}[i=j], \forall i,j$. Under this definition, we have
\begin{align}
    &E_{x\sim q}\set{A}_pk(x,\bar{x})\nonumber\\
   =&\int_{\Omega}\sum_j\lambda_je_j(x)e_j(\bar{x})(\nabla_x \log p(x)-\nabla_x\log q(x))q(x)dx\nonumber\\
    =&\sum_j\lambda_je_j(\bar{x})\int_{\Omega}(\nabla_x \log p(x)-\nabla_x\log q(x))e_j(x)q(x)dx.
    \label{Eq:A2}
\end{align}
Note that $$\set{D}(q\|p)=E_{\bar{x}\sim p}\|E_{x\sim q}\set{A}_pk(x,\bar{x})\|^2=0$$ and $p$ is a positive continuous function over $\Omega$, we have 
$$\forall \bar{x}\in\Omega, E_{x\sim q}\set{A}_pk(x,\bar{x})=0.$$
Let $B_j$ denote $\int_{\Omega}(\nabla_x \log p(x)-\nabla_x\log q(x))e_j(x)q(x)dx$. Applying (\ref{Eq:A2}), we have
$$\forall \bar{x}\in\Omega, \sum_j\lambda_je_j(\bar{x})B_j=0$$
For any $j_0$, we can multiply $e_{j_0}(\bar{x})$ on both sides and then do integral to get
$$\int_{\Omega}e_{j_0}(\bar{x})\sum_j\lambda_je_j(\bar{x})B_j d\bar{x}=0$$
$$\sum_j\lambda_jB_j\int_{\Omega}e_j(\bar{x})e_{j_0}(\bar{x}) d\bar{x}=\lambda_{j_0}B_{j_0}=0$$
Since $\lambda_{j_0}>0$, $B_{j_0}=0$.
Therefore,
\begin{align}
   \forall j_0, \quad \int_{\Omega}\Big(\nabla_x \log p(x)-\nabla_x\log q(x)\Big)e_{j_0}(x)q(x)dx=0\label{Eq:A3}
\end{align}
We can decompose $\Big(\nabla_x \log p(x)-\nabla_x\log q(x)\Big)q(x)$ under the basis $\{e_j\}$ and have
$$\Big(\nabla_x \log p(x)-\nabla_x\log q(x)\Big)q(x)=\sum_jf_je_j(x)$$
holds for some $\{f_j\}$. (\ref{Eq:A3}) can be written as
$$\forall j_0, \int_{\Omega}\sum_j f_je_j(x)e_{j_0}(x)dx=f_{j_0}=0.$$
which implies $$\Big(\nabla_x \log p(x)-\nabla_x\log q(x)\Big)q(x)=0.$$
As $q(x)>0$, we have $$\nabla_x \log p(x)=\nabla_x\log q(x).$$
Therefore, $$\exists C\text{ s.t. }p(x)=Cq(x).$$
Note that both $p$ and $q$ are density functions which implies $\int_{\Omega}p(x)dx=\int_{\Omega}q(x)dx=1$. Thus, $C=1$ which means
$p=q$.
\qed

\section{Details on Permutation Initialization}
\label{App:Prop:2}

It is easy to see that (\ref{Eq:Perm:OPT}) nicely decouples into optimizing the permutations associated each class independently. We proceed to reformulate (\ref{Eq:Perm:OPT}) in its matrix form. Denote $P_j = (P_{1j}^T, \cdots, P_{Nj}^T)^{T}$. Consider block matrix $L \in\R^{Nn_i \times N n_i}$ whose blocks are given by
$$
L_{ii'} = \left\{
\begin{array}{cc}
\sum\limits_{j \neq i} w_{ij} X_{ij}^{T}X_{ij} & i' = i \\
-X_{ij}^{T}X_{i'j} & i'\neq i \\
0 & \textup{otherwise}
\end{array}
\right.\
$$
Then it is clear that (\ref{Eq:Perm:OPT}) is equivalent to solving the following decoupled problems:
\begin{equation}
P_{j}^{\star} = \underset{P_{j}}{\textup{minimize}}\ P_j^{T}\cdot L\cdot P_j.
\label{Eq:Perm:OPT2}
\end{equation}

For general matrix $L$, solving (\ref{Eq:Perm:OPT2}) exactly is NP-hard. In this paper, we use spectral decomposition to find an approximated solution. The motivation comes from the fact that when ${P_j^{\star}}^{T}\cdot L\cdot {P_j^{\star}} = 0$, then $P_{j}^{\star}$ can be derived from spectral decomposition of $L$:
\begin{proposition}
Suppose there exist permutations $P_{ij}^{\star},1\leq j \leq N$ such that
$$
X_{ij}P_{ij}^{\star} = X_{i'j}P_{i'j}^{\star}, \quad \forall 1\leq i\neq i' \leq n.
$$
Let $U = (U_1^{T}, \cdots, U_{N}^{T})^{T}\in R^{n n_i \times n_i}$ be the first $n_i$ eigenvectors of $L$. Then there exists a permutation $P$ so that
$$
P_{ij}^{\star}P = n\cdot U_j\cdot U_1^{T}, \qquad 1\leq i \leq n.
$$
\label{Prop:2}
\end{proposition}
\noindent\textsl{Proof:}
Since the graph $\set{G}$ is connected, it follows that there exists a matrix $M$ so that
$$
X_{ij}P_{ij}^{\star} = M, \quad 1\leq i \leq n.
$$
This means
$$
X_{ij}^{T}X_{i'j} = P_{ij}^{\star}\cdot (M^{T}M)\cdot {P_{i'j}^{\star}}^{T}.
$$
Introduce block-diagonal matrix $P_j = \diag(P_{1j}^{\star},\cdots, P_{nj}^{\star})$. It is easy to see that
$$
L = P_j\big(L_{\set{G}}\otimes (M^{T}M)\big)P_{j}^{T},
$$
where $L_{\set{G}}$ is the graph Laplacian of $\set{G}$. Let $V$ be the eigenvectors of $M^{T}M$. It is easy to see that the top $n_j$ eigenvectors of $L$ is given by (up to a rotation)
$$
U = P_j \cdot (\bs{u}\otimes V).
$$
This means
$$
U_i U_1^{T} = (u_i\cdot u_1)\cdot P_{ij}^{\star}{P_{1j}^{\star}}^{T}, 
$$
which ends the proof.
\qed

In general, $n(U_j U_1^{T})$ is not a permutation matrix. However, we can apply linear assignment to round $n(\cdot U_j\cdot U_1^{T})$ into a permutation by solving a linear assignment:
\begin{equation}
P_{ij}^{\star} = \underset{P}{\min}\|n U_j U_1^{T}  - P\|_{\set{F}}^2 = \underset{P}{\max}\ \textup{Trace}(U_1 U_j^{T}P).
\label{Eq:LA:1}
\end{equation}
In our implementation, we used Hungarian algorithm for solving these linear assignments.

\section{Explicit Expressions for Quasi-Newton Optimization}
\label{App:GN:Method}

To simplify our discussion, we introduce the following notation:
\begin{align*}
\bs{a}_{ki} & := \frac{2}{h}\bs{y}_{k} - (1+\frac{2}{h})\bs{z}_i, & 1\leq i \leq n, 1\leq k \leq L,\\
\bs{b}_{ki} & := \bs{y}_{k} - \bs{z}_i,& 1\leq i \leq n, 1\leq k \leq L,\\
H_{ki} & := (1+\frac{2}{h})I_d - \frac{2}{h}\bs{a}_{ki}\bs{b}_{ki}^{T}, & 1\leq i \leq n, 1\leq k \leq L, \\ 
\bs{c}_{k} & := \sum\limits_{\overline{i} = 1}^{n}\bs{a}_{k\overline{i}}\exp\big(-\frac{\|\bs{b}_{k\overline{i}}\|^2}{h}\big), & 1\leq k \leq L.
\end{align*}

The following proposition provides the explicit expressions of the block diagonal Hessian matrices $H_i$ and the gradient information $\nabla_{\bs{z}_i} f(\bs{z})$: 
\begin{proposition}
The derivatives of $f$ with respect to the coordinates $z_{il}$ of $\bs{z}_i$ are given by 
\begin{align}
&\frac{\partial f}{\partial z_{il}} = -2\textup{Tr}\Big((X_{ij} - G_{\theta}(\bs{z}_i)E_{ij})^{T}\frac{\partial G_{\theta}(\bs{z}_i)}{\partial z_{il}}E_{ij}\Big) \nonumber \\
&\quad -2\sum\limits_{k=1}^{L}\exp\big(-\frac{\|\bs{b}_{ki}\|^2}{h}\big)\bs{e}_l^{T}H_{ki}^{T}\bs{c}_{k}, 
\quad 
\begin{array}{c}
1\leq i \leq n \\
1\leq l \leq n_i.
\end{array}
\label{Eq:Expression:Gradient}
\end{align}

The elements $\bs{e}_{l}^{T}H_i \bs{e}_{\overline{l}}$ of $H_i$ are given by
\begin{align}
\bs{e}_{l}^{T}H_i \bs{e}_{\overline{l}} & = 2 \bs{e}_{l}^{T}\Big(\sum\limits_{k=1}^{L}\exp(-\frac{2\|\bs{b}_{ki}\|^2}{h})H_{ki}^{T}H_{ki}\Big) \bs{e}_{\overline{l}}  \nonumber \\
& + 2\langle \frac{\partial G_{\theta}(\bs{z}_i)}{\partial z_{il}}E_{ij}, \frac{\partial G_{\theta}(\bs{z}_i)}{\partial z_{i\overline{l}}}E_{ij} \rangle,\quad 
\begin{array}{c}
1\leq i \leq n\\
1\leq l, \overline{l}\leq n_i.
\end{array}
\label{Eq:Expression:Hessian}
\end{align}
\end{proposition}
\noindent\textsl{Proof:} We only provide the derivation regarding the derivative of (\ref{Eq:D:Discrete}), since the expression of the data term is trivial. In fact,
\begin{align}
   & \frac{\partial}{\partial \bs{z}_i}\Big(\sum\limits_{i=1}^{n}\bs{a}_{ki}\exp(-\frac{\|\bs{b}_{ki}\|^2}{h})\Big) \nonumber \\
= & \sum\limits_{i=1}^{n}\exp(-\frac{\|\bs{b}_{ki}\|^2}{h})\Big( \frac{\partial \bs{a}_{ki}}{\partial \bs{z}_i}-\frac{2}{h} \bs{a}_{ki}\bs{b}_{ki}^{T}\frac{\partial \bs{b}_{ki}}{\partial \bs{z}_i} \Big) \nonumber \\
= & -\sum\limits_{i=1}^{n}\exp(-\frac{\|\bs{b}_{ki}\|^2}{h})\Big( (1+\frac{2}{h})I_d-\frac{2}{h} \bs{a}_{ki}\bs{b}_{ki}^{T}\Big) \nonumber \\
= & -\sum\limits_{i=1}^{n}\exp(-\frac{\|\bs{b}_{ki}\|^2}{h})H_{ki}.
\label{Eq:Jacobi}
\end{align}
It is easy to check that (\ref{Eq:Expression:Gradient}) and (\ref{Eq:Expression:Hessian}) directly follow from (\ref{Eq:Jacobi}).
\qed
\section{Network Architecture}
\label{App:GN:Method}
\begin{table}[h!]
\centering
\begin{tabular}{ |c|c|c| } 
 \hline
 Type & Layer & \# Units \\ 
 \hline
 \hline
 \multirow{2}{2em}{Type A} & 1 & 512 \\
  & 2-4 & 1024 \\
 \hline
 \multirow{3}{2em}{Type B} & 1,5 & 512 \\ 
 & 2,4 & 256 \\
 & 3 & 128 \\
 \hline
\end{tabular}
\caption{Network Architecture Details}
\label{table:Net}
\end{table}
Table \ref{table:Net} shows the details of hidden layers in our network architecture.

\section{Alternative Formulation of Incorporating a GAN Loss}

\begin{align}
\max\limits_{\phi} \ \min_{\theta, \bs{z}} & \sum\limits_{i=1}^{n}\big( d^2(X_i, \overline{X}_i) + \gamma\|\overline{X}_i- G_{\theta}(\bs{z}_i))\|_{\set{F}}^2 + \lambda \set{D}(\bs{z}, p)\big) \nonumber \\
& + \mu \big(\sum\limits_{i=1}^{n}f_{\phi}(\overline{X}_i)-\sum\limits_{z \in Z_{rand}}f_{\phi}(G_{\theta}(z))\big) 
\end{align}

\section{Formulation of Incorporating an auto-encoder}

\begin{equation}
\underset{\theta}{\min} \ \sum\limits_{i=1}^{n} \sum\limits_{j=1}^{m} \underset{P_{ij} \in \set{P}_{nj}}{\min}\|X_{ij} - (AE_\theta(X_{ij})E_j)\cdot(M_{ij}P_{ij})\|_{\set{F}}^2
\end{equation},
where $\theta$ is the network parameters, and $\set{P}_{n_j}$ denotes the space of permutations of dimension $n_j$, $E_{j} = (0, \cdots, I_{n_i}, \cdots, 0)^{T}$ is the matrix that extracts the corresponding sub-matrix of $AE_\theta(X_{ij})$, and $P_{ij}$ is the permutation matrix for the sub-matrix. $M_{ij} \in [0,1]^{\overline{d}\times n_j}$ is the mask matrix, where the first row is always $1$, and the remaining elements of each column are set to $0$ if the corresponding object is not selected, otherwise the remaining elements are set to $1$.

\section{Qixing's Formulation}
Suppose we have $n$ scenes encoded as $X_1, \cdots, X_{n}$, where $X_{i}\in \R^{km\times d}$. Here $k$ is the maximum number of objects per category, $m$ is the total number of categories, and $d$ is the dimension of the encoding. To factor out the encoding, we associated each scene with a latent variable $\theta_i$. In our case, $\theta_i$ collects the permutation associated with each category, and the global rotation and translation associated with scene. We also introduce a function $f(\theta, X)\in \R^{km\times d}$, which takes a latent parameter $\theta$ and a scene as input, and outputs the permuted scene. Note that $f$ is predefined. 

Our goal is to train an auto-encoder $G_{\phi}: \R^{km\times d}\rightarrow \R^{km\times d}$ by minimizing the following objective function:
\begin{equation}
\underset{\{\theta_i, Y_i, 1\leq i \leq n\}, \phi}{\textup{minimize}}\ \sum\limits_{i=1}^{n}\|Y_i -G_{\phi}(Y_i)\|_{\set{F}}^2 + \lambda \sum\limits_{i=1}^{n}\|f(\theta_i, X_i) - Y_i\|_{\set{F}}^2 
\label{Eq:Total:Obj}
\end{equation}
where $Y_i\in \R^{km\times d}$ are latent variables. (\ref{Eq:Total:Obj}) can be easily solved via alternating minimization. Specifically, we can fix $Y_i$ and $\theta_i$ to optimize $\phi$. We can then fix $\phi$ to optimize $Y_i$ and $\theta_i$.

\section{Regularization on Objects Pairwise Distance}
Our goal is to train an auto-encoder $G_{\phi}: \R^{km\times d}\rightarrow \R^{km\times d}$ by minimizing the following objective function:
\begin{align}
\underset{\{\theta_i, Y_i, 1\leq i \leq n\}, \phi}{\textup{minimize}}\ & \sum\limits_{i=1}^{n}\|Y_i -G_{\phi}(Y_i)\|_{\set{F}}^2 + \lambda \sum\limits_{i=1}^{n}\|f(\theta_i, X_i) - Y_i\|_{\set{F}}^2  \nonumber \\ 
& + \beta \sum\limits_{i=1}^{n} D_{KL}(P(Z_i),P(f(\theta_i, X_i)))  \nonumber
\end{align}
where $Y_i\in \R^{km\times d}$ are latent variables, $P(\cdot)$ is a function calculating pairwise distance matrix for location, size and orientation, $Z_i$ are generated scenes based on slightly perturbed middle embedding of $Y_i$ and $D_{KL} = \sum\limits_{k,l=1}^{m}Z_i(k,l)\log\frac{Z_i(k,l)}{f(\theta_i, X_i)(k,l)}$.

\section{Current Regularization}
\begin{align}
\underset{\{\theta_i, Y_i, 1\leq i \leq n\}, \phi}{\textup{minimize}}\ & \sum\limits_{i=1}^{n}\|Y_i -G_{\phi}(Y_i)\|_{\set{F}}^2 + \lambda \sum\limits_{i=1}^{n}\|f(\theta_i, X_i) - Y_i\|_{\set{F}}^2  \nonumber \\ 
& + \beta \sum\limits_{i=1}^{n}\|f(\theta_i, X_i) - Z_i\|_{\set{F}}^2 \nonumber
\end{align}
where $Z_i$ are generated scenes based on slightly perturbed middle embedding of $Y_i$.

\newpage
 \\
\newpage

\section{Current Formulation}

\begin{align}
\underset{\theta_3}{\max}\underset{\theta_1, \theta_2, P, P*}{\min} & \ \frac{\alpha}{n}\sum\limits_{i=1}^{n} \sum\limits_{j=1}^{m} \underset{P_{ij} \in \set{P}_{nj}}{\min}\|X_{ij} - (G_{\theta_2}(En_{\theta_1}(X_{ij}))E_j)\cdot(M_{ij}P_{ij})\|_{\set{F}}^2 \nonumber \\
& + \frac{\beta}{n} \big(\sum\limits_{i=1}^{n}D_{\theta_3}(X_{i}\cdot P^*_{i})-\sum\limits_{z \in Z_{rand}}D_{\theta_3}(G_{\theta_2}(z) \cdot M_i)\big) \nonumber \\
& + \phi L(En_{\theta_1}(X_{ij}))
\end{align},
where $\alpha$, $\beta$, and $\phi$ are constants, and $L(\cdot)$ is a latent loss term, which is the KL-divergence between middle embedding and unit normal distribution. $\theta_1$ is the network parameters for encoder, $\theta_2$ is the network parameters for decoder and $\theta_3$ is the network parameters for discriminator, and $\set{P}_{n_j}$ denotes the space of permutations of dimension $n_j$, $E_{j} = (0, \cdots, I_{n_i}, \cdots, 0)^{T}$ is the matrix that extracts the corresponding sub-matrix of the reconstructed scene matrices, and $P_{ij}$ is the permutation matrix for the sub-matrix. $M_{ij} \in [0,1]^{\overline{d}\times n_j}$ is the mask matrix, where the first row is always $1$, and the remaining elements of each column are set to $0$ if the corresponding object is not selected, otherwise the remaining elements are set to $1$. $P^*$ is a permutation matrix and optimized using the following energy function:
\begin{align}
\underset{P*}{\min} & \sum\limits_{i=1}^{n} \big((X_{i}\cdot P^*_{i})-(G(z_{\mathbf{N}(0,I)})))
\end{align}
, where z is drawn from normal distribution.
