# Supplementary material for: Deep Generative Modeling for Scene Synthesis via Hybrid Representations
Source: arXiv:1808.02084 source file (2018-08-06)
Supplement: Supplementary file 2 [file 09_appendix_A.tex]

\section{Stein Discrepancy}
\label{Sec:Distance}

In this section, we provide a detailed introduction of the proposed Stein discrepancy measurement used in this paper.
We start with the Stein operator, which provides the foundation for our continuous formulation.
\begin{defn}
Given a function $f(\bs{x})$ and a smooth probability distribution $p(\bs{x})$ over a space $\Omega$, we define the Stein operator on $f(\bs{x})$ as
$$
\set{A}_{p}f(\bs{x}):= \nabla \log(p(\bs{x}))f(\bs{x}) + \nabla_{\bs{x}} f(\bs{x}).
$$
\end{defn}

We then define the notion of the \textsl{Stein} class of a probability distribution, which will be used later:
\begin{defn}
Given a space $\Omega$ and probability distribution $p(\bs{x})$ over $\Omega$, we say a function $f(\bs{x})$ is in the Stein class of $p(\bs{x})$ if
$$
\int_{\Omega}\nabla_{\bs{x}}(f(\bs{x})p(\bs{x})) = 0.
$$
\label{Defn:Stein:Class}
\end{defn}
In the case $\Omega = \R^d$, one condition that holds for Definition (\ref{Defn:Stein:Class}) is that $f(\bs{x})p(\bs{x}) = 0$ when $\|\bs{x}\|\rightarrow \infty$. For example, the kernel function $k(\bs{x},\bs{z}) = \exp(-\frac{\|\bs{x}-\bs{z}\|^2}{h})$ for fixed $\bs{z}$ is the Stein class of the normal distribution.

Now we introduce an important property of the Stein operator:
\begin{prop}
If $f(\bs{x})$ is in the Stein class of $p(\bs{x})$, then
\begin{equation}
E_{x\sim p}\big(\set{A}_{p}f\big)(\bs{x}) := \int_{\Omega}\set{A}_{p}f(\bs{x}) \cdot p(\bs{x}) d\bs{x} = 0.
\label{Eq:Stein}
\end{equation}
\end{prop}
\noindent\textsl{Proof:}
\begin{align}
E_{x\sim p}\big(\set{A}_{p}f\big)(\bs{x}) & = \int_{\Omega}\big(\nabla \log{p(\bs{x})} f(\bs{x}) + \nabla f(\bs{x})\big)p(\bs{x}) d\bs{x}  \nonumber \\
& = \int_{\Omega}\big(\nabla p(\bs{x}) f(\bs{x}) + \nabla f(\bs{x}) p(\bs{x}) \big)d\bs{x} \nonumber \\
& = \int_{\Omega} \nabla_{\bs{x}}(p(\bs{x})f(\bs{x}))d\bs{x} = 0.
\end{align}
\qed

(\ref{Eq:Stein}) provides a powerful tool to access the difference between two distributions $p$ and $q$, namely, $E_{x\sim q}\big(\set{A}_{p}f\big)(\bs{x}) =0$ would not hold when $q \neq p$. To convert this intuition into a distance measure, we utilize a positive definite kernel function $k(\bs{x}, \bs{x}')$ and define:
\begin{equation}
\set{D}(q||p) := E_{\overline{\bs{x}}\sim p}\|E_{x\sim q}A_{p}k(\bs{x},\overline{\bs{x}})\|^2.
\label{Eq:D}
\end{equation}

We can show that under mild conditions of $p$ and $q$. $\set{D}(q||p) = 0$ if and only if $p = q$, which means $\set{D}$ provides a meaningful distance measure between probability distributions. To formalize this, we need to define the reproducing kernel Hilbert space of a kernel:
\begin{definition}
Let $k(\bs{x},\bs{x}'):\Omega \times \Omega \rightarrow \R^{+}$ be a positive definite kernel. The reproducing kernel Hilbert space (RKHS) $\set{H}$ of $k(\bs{x},\bs{x}')$ is the closure of the linear span $\{f:f(\bs{x}):= \sum_{i=1}^{m}a_i k(\bs{x}, \bs{x}_i), a_i \in \R, m \geq 0, \bs{x}\in \Omega\}$, equipped with inner products $<f.g>_{H} = \sum_{ij}a_i b_j k(\bs{x}_i, \bs{x}_j)$ for $g(\bs{x}) = \sum_i b_i k(\bs{x}, \bs{x}_i)$.
\end{definition}

\begin{prop}
Given a positive definite kernel $k$ and the associated reproducing kernel Hilbert space $\set{H}$. Suppose $p,q \in \set{H}$. Then
$$
\set{D}(q||p) = 0 \qquad \textup{iff} \qquad q = p.
$$
\label{Prop:1}
\end{prop}

\noindent\textsl{Proof:} Since $k(x,x')$ is in the stain class of $p$, $k(\cdot,\bar{x})$ is in the stain class of $p$ which implies $E_{x\sim p}\set{A}_pk(x,\bar{x})=0$ for all $\bar{x}\in \Omega$. Therefore, if $p=q$, $\set{D}(q\|p)=0$. We only need to show $p=q$ if $\set{D}(q\|p)=0$.

Note that $k(x,x')$ is in the Stein class of $q$ and $q$ is a smooth density function. We have for any fixed $\bar{x}\in\Omega$,
\begin{align}
   &\int_{\Omega}\nabla_x(k(x,\bar{x})q(x))dx\nonumber\\
   =&\int_{\Omega}(k(x,\bar{x})\nabla_x \log q(x)+\nabla_x k(x,\bar{x}))q(x) dx=0
   \label{Eq:A1}
\end{align}
By applying Proposition(1) and (\ref{Eq:A1}), we have
\begin{align}
   &E_{x\sim q}\set{A}_pk(x,\bar{x})\nonumber\\
   =&\int_{\Omega}\set{A}_pk(x,\bar{x})q(x)dx\nonumber\\
   =&\int_{\Omega}((\nabla_x\log p(x))k(x,\bar{x})+\nabla_xk(x,\bar{x}))q(x) dx\nonumber\\
   =&\int_{\Omega}(\nabla_x\log p(x)-\nabla_x\log q(x))k(x,\bar{x})q(x) dx.\nonumber
\end{align}

We can do spectral decomposition of $k(x,x')$, as implied by Mercer's theorem, to get
$$k(x,x')=\sum_j\lambda_je_j(x)e_j(x'),$$
where $\{e_j\}\{\lambda_j\}$ are the orthonormal eigenfunctions and positive eigenvalues of $k(x,x')$, satisfying $\int_\Omega e_i(x)e_j(x)dx=\mathbb{I}[i=j], \forall i,j$. Under this definition, we have
\begin{align}
    &E_{x\sim q}\set{A}_pk(x,\bar{x})\nonumber\\
   =&\int_{\Omega}\sum_j\lambda_je_j(x)e_j(\bar{x})(\nabla_x \log p(x)-\nabla_x\log q(x))q(x)dx\nonumber\\
    =&\sum_j\lambda_je_j(\bar{x})\int_{\Omega}(\nabla_x \log p(x)-\nabla_x\log q(x))e_j(x)q(x)dx.
    \label{Eq:A2}
\end{align}
Note that $$\set{D}(q\|p)=E_{\bar{x}\sim p}\|E_{x\sim q}\set{A}_pk(x,\bar{x})\|^2=0$$ and $p$ is a positive continuous function over $\Omega$, we have 
$$\forall \bar{x}\in\Omega, E_{x\sim q}\set{A}_pk(x,\bar{x})=0.$$
Let $B_j$ denote $\int_{\Omega}(\nabla_x \log p(x)-\nabla_x\log q(x))e_j(x)q(x)dx$. Applying (\ref{Eq:A2}), we have
$$\forall \bar{x}\in\Omega, \sum_j\lambda_je_j(\bar{x})B_j=0$$
For any $j_0$, we can multiply $e_{j_0}(\bar{x})$ on both sides and then do integral to get
$$\int_{\Omega}e_{j_0}(\bar{x})\sum_j\lambda_je_j(\bar{x})B_j d\bar{x}=0$$
$$\sum_j\lambda_jB_j\int_{\Omega}e_j(\bar{x})e_{j_0}(\bar{x}) d\bar{x}=\lambda_{j_0}B_{j_0}=0$$
Since $\lambda_{j_0}>0$, $B_{j_0}=0$.
Therefore,
\begin{align}
   \forall j_0, \quad \int_{\Omega}\Big(\nabla_x \log p(x)-\nabla_x\log q(x)\Big)e_{j_0}(x)q(x)dx=0\label{Eq:A3}
\end{align}
We can decompose $\Big(\nabla_x \log p(x)-\nabla_x\log q(x)\Big)q(x)$ under the basis $\{e_j\}$ and have
$$\Big(\nabla_x \log p(x)-\nabla_x\log q(x)\Big)q(x)=\sum_jf_je_j(x)$$
holds for some $\{f_j\}$. (\ref{Eq:A3}) can be written as
$$\forall j_0, \int_{\Omega}\sum_j f_je_j(x)e_{j_0}(x)dx=f_{j_0}=0.$$
which implies $$\Big(\nabla_x \log p(x)-\nabla_x\log q(x)\Big)q(x)=0.$$
As $q(x)>0$, we have $$\nabla_x \log p(x)=\nabla_x\log q(x).$$
Therefore, $$\exists C\text{ s.t. }p(x)=Cq(x).$$
Note that both $p$ and $q$ are density functions which implies $\int_{\Omega}p(x)dx=\int_{\Omega}q(x)dx=1$. Thus, $C=1$ which means
$p=q$.
\qed
