# Supplementary material for: Deep Generative Modeling for Scene Synthesis via Hybrid Representations
Source: arXiv:1808.02084 source file (2018-08-06)
Supplement: Supplementary file 3 [file 09_appendix_B.tex]

\section{Details on Permutation Initialization}
\label{App:Prop:2}

It is easy to see that (\ref{Eq:Perm:OPT}) nicely decouples into optimizing the permutations associated each class independently. We proceed to reformulate (\ref{Eq:Perm:OPT}) in its matrix form. Denote $P_j = (P_{1j}^T, \cdots, P_{Nj}^T)^{T}$. Consider block matrix $L \in\R^{Nn_i \times N n_i}$ whose blocks are given by
$$
L_{ii'} = \left\{
\begin{array}{cc}
\sum\limits_{j \neq i} w_{ij} X_{ij}^{T}X_{ij} & i' = i \\
-X_{ij}^{T}X_{i'j} & i'\neq i \\
0 & \textup{otherwise}
\end{array}
\right.\
$$
Then it is clear that (\ref{Eq:Perm:OPT}) is equivalent to solving the following decoupled problems:
\begin{equation}
P_{j}^{\star} = \underset{P_{j}}{\textup{minimize}}\ P_j^{T}\cdot L\cdot P_j.
\label{Eq:Perm:OPT2}
\end{equation}

For general matrix $L$, solving (\ref{Eq:Perm:OPT2}) exactly is NP-hard. In this paper, we use spectral decomposition to find an approximated solution. The motivation comes from the fact that when ${P_j^{\star}}^{T}\cdot L\cdot {P_j^{\star}} = 0$, then $P_{j}^{\star}$ can be derived from spectral decomposition of $L$:
\begin{proposition}
Suppose there exist permutations $P_{ij}^{\star},1\leq j \leq N$ such that
$$
X_{ij}P_{ij}^{\star} = X_{i'j}P_{i'j}^{\star}, \quad \forall 1\leq i\neq i' \leq n.
$$
Let $U = (U_1^{T}, \cdots, U_{N}^{T})^{T}\in R^{n n_i \times n_i}$ be the first $n_i$ eigenvectors of $L$. Then there exists a permutation $P$ so that
$$
P_{ij}^{\star}P = n\cdot U_j\cdot U_1^{T}, \qquad 1\leq i \leq n.
$$
\label{Prop:2}
\end{proposition}
\noindent\textsl{Proof:}
Since the graph $\set{G}$ is connected, it follows that there exists a matrix $M$ so that
$$
X_{ij}P_{ij}^{\star} = M, \quad 1\leq i \leq n.
$$
This means
$$
X_{ij}^{T}X_{i'j} = P_{ij}^{\star}\cdot (M^{T}M)\cdot {P_{i'j}^{\star}}^{T}.
$$
Introduce block-diagonal matrix $P_j = \diag(P_{1j}^{\star},\cdots, P_{nj}^{\star})$. It is easy to see that
$$
L = P_j\big(L_{\set{G}}\otimes (M^{T}M)\big)P_{j}^{T},
$$
where $L_{\set{G}}$ is the graph Laplacian of $\set{G}$. Let $V$ be the eigenvectors of $M^{T}M$. It is easy to see that the top $n_j$ eigenvectors of $L$ is given by (up to a rotation)
$$
U = P_j \cdot (\bs{u}\otimes V).
$$
This means
$$
U_i U_1^{T} = (u_i\cdot u_1)\cdot P_{ij}^{\star}{P_{1j}^{\star}}^{T}, 
$$
which ends the proof.
\qed

In general, $n(U_j U_1^{T})$ is not a permutation matrix. However, we can apply linear assignment to round $n(\cdot U_j\cdot U_1^{T})$ into a permutation by solving a linear assignment:
\begin{equation}
P_{ij}^{\star} = \underset{P}{\min}\|n U_j U_1^{T}  - P\|_{\set{F}}^2 = \underset{P}{\max}\ \textup{Trace}(U_1 U_j^{T}P).
\label{Eq:LA:1}
\end{equation}
In our implementation, we used Hungarian algorithm for solving these linear assignments.
