# Supplementary material for: Deep Generative Modeling for Scene Synthesis via Hybrid Representations
Source: arXiv:1808.02084 source file (2018-08-06)
Supplement: Supplementary file 4 [file 09_appendix_C.tex]

\section{Explicit Expressions for Quasi-Newton Optimization}
\label{App:GN:Method}

To simplify our discussion, we introduce the following notation:
\begin{align*}
\bs{a}_{ki} & := \frac{2}{h}\bs{y}_{k} - (1+\frac{2}{h})\bs{z}_i, & 1\leq i \leq n, 1\leq k \leq L,\\
\bs{b}_{ki} & := \bs{y}_{k} - \bs{z}_i,& 1\leq i \leq n, 1\leq k \leq L,\\
H_{ki} & := (1+\frac{2}{h})I_d - \frac{2}{h}\bs{a}_{ki}\bs{b}_{ki}^{T}, & 1\leq i \leq n, 1\leq k \leq L, \\ 
\bs{c}_{k} & := \sum\limits_{\overline{i} = 1}^{n}\bs{a}_{k\overline{i}}\exp\big(-\frac{\|\bs{b}_{k\overline{i}}\|^2}{h}\big), & 1\leq k \leq L.
\end{align*}

The following proposition provides the explicit expressions of the block diagonal Hessian matrices $H_i$ and the gradient information $\nabla_{\bs{z}_i} f(\bs{z})$: 
\begin{proposition}
The derivatives of $f$ with respect to the coordinates $z_{il}$ of $\bs{z}_i$ are given by 
\begin{align}
&\frac{\partial f}{\partial z_{il}} = -2\textup{Tr}\Big((X_{ij} - G_{\theta}(\bs{z}_i)E_{ij})^{T}\frac{\partial G_{\theta}(\bs{z}_i)}{\partial z_{il}}E_{ij}\Big) \nonumber \\
&\quad -2\sum\limits_{k=1}^{L}\exp\big(-\frac{\|\bs{b}_{ki}\|^2}{h}\big)\bs{e}_l^{T}H_{ki}^{T}\bs{c}_{k}, 
\quad 
\begin{array}{c}
1\leq i \leq n \\
1\leq l \leq n_i.
\end{array}
\label{Eq:Expression:Gradient}
\end{align}

The elements $\bs{e}_{l}^{T}H_i \bs{e}_{\overline{l}}$ of $H_i$ are given by
\begin{align}
\bs{e}_{l}^{T}H_i \bs{e}_{\overline{l}} & = 2 \bs{e}_{l}^{T}\Big(\sum\limits_{k=1}^{L}\exp(-\frac{2\|\bs{b}_{ki}\|^2}{h})H_{ki}^{T}H_{ki}\Big) \bs{e}_{\overline{l}}  \nonumber \\
& + 2\langle \frac{\partial G_{\theta}(\bs{z}_i)}{\partial z_{il}}E_{ij}, \frac{\partial G_{\theta}(\bs{z}_i)}{\partial z_{i\overline{l}}}E_{ij} \rangle,\quad 
\begin{array}{c}
1\leq i \leq n\\
1\leq l, \overline{l}\leq n_i.
\end{array}
\label{Eq:Expression:Hessian}
\end{align}
\end{proposition}
\noindent\textsl{Proof:} We only provide the derivation regarding the derivative of (\ref{Eq:D:Discrete}), since the expression of the data term is trivial. In fact,
\begin{align}
   & \frac{\partial}{\partial \bs{z}_i}\Big(\sum\limits_{i=1}^{n}\bs{a}_{ki}\exp(-\frac{\|\bs{b}_{ki}\|^2}{h})\Big) \nonumber \\
= & \sum\limits_{i=1}^{n}\exp(-\frac{\|\bs{b}_{ki}\|^2}{h})\Big( \frac{\partial \bs{a}_{ki}}{\partial \bs{z}_i}-\frac{2}{h} \bs{a}_{ki}\bs{b}_{ki}^{T}\frac{\partial \bs{b}_{ki}}{\partial \bs{z}_i} \Big) \nonumber \\
= & -\sum\limits_{i=1}^{n}\exp(-\frac{\|\bs{b}_{ki}\|^2}{h})\Big( (1+\frac{2}{h})I_d-\frac{2}{h} \bs{a}_{ki}\bs{b}_{ki}^{T}\Big) \nonumber \\
= & -\sum\limits_{i=1}^{n}\exp(-\frac{\|\bs{b}_{ki}\|^2}{h})H_{ki}.
\label{Eq:Jacobi}
\end{align}
It is easy to check that (\ref{Eq:Expression:Gradient}) and (\ref{Eq:Expression:Hessian}) directly follow from (\ref{Eq:Jacobi}).
\qed
