# Supplementary material for: Deep Generative Modeling for Scene Synthesis via Hybrid Representations
Source: arXiv:1808.02084 source file (2018-08-06)
Supplement: Supplementary file 5 [file 09_appendix_D.tex]

\section{Network Architecture}
\label{App:GN:Method}
\begin{table}[h!]
\centering
\begin{tabular}{ |c|c|c| } 
 \hline
 Type & Layer & \# Units \\ 
 \hline
 \hline
 \multirow{2}{2em}{Type A} & 1 & 512 \\
  & 2-4 & 1024 \\
 \hline
 \multirow{3}{2em}{Type B} & 1,5 & 512 \\ 
 & 2,4 & 256 \\
 & 3 & 128 \\
 \hline
\end{tabular}
\caption{Network Architecture Details}
\label{table:Net}
\end{table}
Table \ref{table:Net} shows the details of hidden layers in our network architecture.
