# Supplementary material for: Deep Generative Modeling for Scene Synthesis via Hybrid Representations
Source: arXiv:1808.02084 source file (2018-08-06)
Supplement: Supplementary file 6 [file 09_appendix_E.tex]

\section{Alternative Formulation of Incorporating a GAN Loss}

\begin{align}
\max\limits_{\phi} \ \min_{\theta, \bs{z}} & \sum\limits_{i=1}^{n}\big( d^2(X_i, \overline{X}_i) + \gamma\|\overline{X}_i- G_{\theta}(\bs{z}_i))\|_{\set{F}}^2 + \lambda \set{D}(\bs{z}, p)\big) \nonumber \\
& + \mu \big(\sum\limits_{i=1}^{n}f_{\phi}(\overline{X}_i)-\sum\limits_{z \in Z_{rand}}f_{\phi}(G_{\theta}(z))\big) 
\end{align}

\section{Formulation of Incorporating an auto-encoder}

\begin{equation}
\underset{\theta}{\min} \ \sum\limits_{i=1}^{n} \sum\limits_{j=1}^{m} \underset{P_{ij} \in \set{P}_{nj}}{\min}\|X_{ij} - (AE_\theta(X_{ij})E_j)\cdot(M_{ij}P_{ij})\|_{\set{F}}^2
\end{equation},
where $\theta$ is the network parameters, and $\set{P}_{n_j}$ denotes the space of permutations of dimension $n_j$, $E_{j} = (0, \cdots, I_{n_i}, \cdots, 0)^{T}$ is the matrix that extracts the corresponding sub-matrix of $AE_\theta(X_{ij})$, and $P_{ij}$ is the permutation matrix for the sub-matrix. $M_{ij} \in [0,1]^{\overline{d}\times n_j}$ is the mask matrix, where the first row is always $1$, and the remaining elements of each column are set to $0$ if the corresponding object is not selected, otherwise the remaining elements are set to $1$.

\section{Qixing's Formulation}
Suppose we have $n$ scenes encoded as $X_1, \cdots, X_{n}$, where $X_{i}\in \R^{km\times d}$. Here $k$ is the maximum number of objects per category, $m$ is the total number of categories, and $d$ is the dimension of the encoding. To factor out the encoding, we associated each scene with a latent variable $\theta_i$. In our case, $\theta_i$ collects the permutation associated with each category, and the global rotation and translation associated with scene. We also introduce a function $f(\theta, X)\in \R^{km\times d}$, which takes a latent parameter $\theta$ and a scene as input, and outputs the permuted scene. Note that $f$ is predefined. 

Our goal is to train an auto-encoder $G_{\phi}: \R^{km\times d}\rightarrow \R^{km\times d}$ by minimizing the following objective function:
\begin{equation}
\underset{\{\theta_i, Y_i, 1\leq i \leq n\}, \phi}{\textup{minimize}}\ \sum\limits_{i=1}^{n}\|Y_i -G_{\phi}(Y_i)\|_{\set{F}}^2 + \lambda \sum\limits_{i=1}^{n}\|f(\theta_i, X_i) - Y_i\|_{\set{F}}^2 
\label{Eq:Total:Obj}
\end{equation}
where $Y_i\in \R^{km\times d}$ are latent variables. (\ref{Eq:Total:Obj}) can be easily solved via alternating minimization. Specifically, we can fix $Y_i$ and $\theta_i$ to optimize $\phi$. We can then fix $\phi$ to optimize $Y_i$ and $\theta_i$.

\section{Regularization on Objects Pairwise Distance}
Our goal is to train an auto-encoder $G_{\phi}: \R^{km\times d}\rightarrow \R^{km\times d}$ by minimizing the following objective function:
\begin{align}
\underset{\{\theta_i, Y_i, 1\leq i \leq n\}, \phi}{\textup{minimize}}\ & \sum\limits_{i=1}^{n}\|Y_i -G_{\phi}(Y_i)\|_{\set{F}}^2 + \lambda \sum\limits_{i=1}^{n}\|f(\theta_i, X_i) - Y_i\|_{\set{F}}^2  \nonumber \\ 
& + \beta \sum\limits_{i=1}^{n} D_{KL}(P(Z_i),P(f(\theta_i, X_i)))  \nonumber
\end{align}
where $Y_i\in \R^{km\times d}$ are latent variables, $P(\cdot)$ is a function calculating pairwise distance matrix for location, size and orientation, $Z_i$ are generated scenes based on slightly perturbed middle embedding of $Y_i$ and $D_{KL} = \sum\limits_{k,l=1}^{m}Z_i(k,l)\log\frac{Z_i(k,l)}{f(\theta_i, X_i)(k,l)}$.

\section{Current Regularization}
\begin{align}
\underset{\{\theta_i, Y_i, 1\leq i \leq n\}, \phi}{\textup{minimize}}\ & \sum\limits_{i=1}^{n}\|Y_i -G_{\phi}(Y_i)\|_{\set{F}}^2 + \lambda \sum\limits_{i=1}^{n}\|f(\theta_i, X_i) - Y_i\|_{\set{F}}^2  \nonumber \\ 
& + \beta \sum\limits_{i=1}^{n}\|f(\theta_i, X_i) - Z_i\|_{\set{F}}^2 \nonumber
\end{align}
where $Z_i$ are generated scenes based on slightly perturbed middle embedding of $Y_i$.

\newpage
 \\
\newpage

\section{Current Formulation}

\begin{align}
\underset{\theta_3}{\max}\underset{\theta_1, \theta_2, P, P*}{\min} & \ \frac{\alpha}{n}\sum\limits_{i=1}^{n} \sum\limits_{j=1}^{m} \underset{P_{ij} \in \set{P}_{nj}}{\min}\|X_{ij} - (G_{\theta_2}(En_{\theta_1}(X_{ij}))E_j)\cdot(M_{ij}P_{ij})\|_{\set{F}}^2 \nonumber \\
& + \frac{\beta}{n} \big(\sum\limits_{i=1}^{n}D_{\theta_3}(X_{i}\cdot P^*_{i})-\sum\limits_{z \in Z_{rand}}D_{\theta_3}(G_{\theta_2}(z) \cdot M_i)\big) \nonumber \\
& + \phi L(En_{\theta_1}(X_{ij}))
\end{align},
where $\alpha$, $\beta$, and $\phi$ are constants, and $L(\cdot)$ is a latent loss term, which is the KL-divergence between middle embedding and unit normal distribution. $\theta_1$ is the network parameters for encoder, $\theta_2$ is the network parameters for decoder and $\theta_3$ is the network parameters for discriminator, and $\set{P}_{n_j}$ denotes the space of permutations of dimension $n_j$, $E_{j} = (0, \cdots, I_{n_i}, \cdots, 0)^{T}$ is the matrix that extracts the corresponding sub-matrix of the reconstructed scene matrices, and $P_{ij}$ is the permutation matrix for the sub-matrix. $M_{ij} \in [0,1]^{\overline{d}\times n_j}$ is the mask matrix, where the first row is always $1$, and the remaining elements of each column are set to $0$ if the corresponding object is not selected, otherwise the remaining elements are set to $1$. $P^*$ is a permutation matrix and optimized using the following energy function:
\begin{align}
\underset{P*}{\min} & \sum\limits_{i=1}^{n} \big((X_{i}\cdot P^*_{i})-(G(z_{\mathbf{N}(0,I)})))
\end{align}
, where z is drawn from normal distribution.
